# Supplementary material for: Script-Based Dialog Policy Planning for LLM-Powered Conversational Agents: A Basic Architecture for an "AI Therapist"
Source: arXiv:2412.15242 source file (2024-12-13)
Supplement: Supplementary file 1 [file Technical_Appendix.pdf]

# Technical Appendix

**Script-Based Dialog Policy Planning for LLM-Powered Conversational Agents: A Basic Architecture for an "AI Therapist"**

**Robert Wasenmüller[1], Kevin Hilbert[2], Christoph Benzmüller[3,4]**
[1]Aury, Berlin, Germany
[2]Department of Psychology, HMU Health and Medical University Erfurt, Erfurt, Germany,
[3]AI Systems Engineering, Otto-Friedrich Universität Bamberg, Bamberg, Germany
[4]Department of Mathematics and Computer Science, Freie Universität Berlin, Berlin, Germany
robert.wasenmueller@aury.co, kevin.hilbert@hmu-erfurt.de, christoph.benzmueller@uni-bamberg.de

August 2024

## A Examples Illustrating the Benefit of Section-Level Instructions

The examples below are intended to demonstrate our claim from Section 2.3 of the paper stating that the Dialog LLM needs *section-level instructions*, i.e. multiple tasks at once, to allow for a more fluent conversation with the user. In both examples, an Actor LLM is assigning task-level instructions, i.e. a single task in each turn, to the Dialog LLM, and expecting it to complete those in a single turn.

In **Example 1**, the Dialog LLM receives an instruction to ask the patient for their name. However, the patient happens to have introduced themselves in the previous turn already. The Dialog LLM doesn't have the freedom to navigate across mutliple tasks, and is forced to adhere to the received task. Hence, it asks the patient for their name again. With *section-level* instructions, the Dialog LLM would have had the freedom to skip this task.

- User: Hi
- Actor LLM: (SYSTEM MESSAGE: Your next task is: Welcome the patient warmly and introduce yourself. Let them know that you are an AI Therapist here to support them.)
- Dialog LLM: Welcome to our session. Im your AI Therapist to support you.
- User: Thanks. You can call me Pete.
- Actor LLM: (SYSTEM MESSAGE: Your next task is: Ask the patient what name they prefer to be called by and wait for their response.
- Dialog LLM: What name would you prefer to be called by?

In **Example 2**, the patient is particularly asking for a CBT exercise which is not part of the Dialog LLM's instructions at this point. Instead, the Dialog LLM strictly follows its task and reacts empathically, but doesn't follow the patient's utterance. With *section-level* instructions, the Dialog LLM would have had the freedom to first react to the patient's utterance and then return to completing its series of tasks.

- Actor LLM: (SYSTEM MESSAGE: Your next task is: Ask the patient how they are doing today and wait for their response.)
- Dialog LLM: How are you doing today, Pete?
- User: Not that good. Actually, can you show me a CBT exercise to tackle my stress?
- Actor LLM: (SYSTEM MESSAGE: Your next task is: React appropriately to the patient's response, showing empathy and understanding.)
- Dialog LLM: Sorry to hear that youre feeling stressed.
- User: What about the CBT exercise?
- Actor LLM: (SYSTEM MESSAGE: Your next task is: Ask the patient whether they would like to further explore what they just told you [then proceed with Section 3] or whether they would like to continue the topic from the last session [then proceed with Section 4], and wait for their response.)
- Dialog LLM: Sure, lets have a closer look at your stress and select a suitable CBT exercise. ...

## B Pseudocode of the Experiments Implementation

This section shows pseudocode representing the high-level structure of the algorithms used to run the experiments, as referenced in section 3 of the main paper.

Algorithm 1 shows pseudocode of the wrapper *run_experiments()* iterating through all relevant cases and calling *run_experiment()* to run each experiment with the respective parameters.

Algorithm 2 shows pseudocode of *run_experiment()*, a recursive function generating all relevant actors' messages on each iteration, and respectively differentiating implementation variants A and B.

## C Exemplary Script

This Section shows the whole exemplary script used in our experiments, as referenced in Figure 2 and Subsection 3.1 of the main paper.

```
{
  "Section 1": {
```

**Algorithm 1**: Wrapper run_experiments() running all experiments

**Input**: Sets of implementation variants, patient cases, and number of experiment runs
**Output**: Evaluation metrics for each experiment run

```
for each implementation_variant from [A, B] do
    for each patient_case from [1, 2, 3, 4, 5] do
        for each experiment_run from [1 to 10] do
            run_experiment(implementation_variant, patient_case)
            compute_evaluation_metrics()
        end for
    end for
end for
return evaluation_metrics
```

```
    "Task 1a": "Welcome the patient warmly and introduce yourself. Let them know your name, and that you are an AI Therapist here to support them.",
    "Task 1b": "Ask the patient what name they prefer to be called by and wait for their response.",
    "Task 1c": "Ask the patient if they have any questions about the service or about you, and answer any questions they might have. Proceed with Section 2 if they don't have any more questions."
  },
  "Section 2": {
    "Task 2a": "Ask the patient how they are doing today and wait for their response.",
    "Task 2b": "React appropriately to the patient's response, showing empathy and understanding. Ask a follow-up question to explore their current emotional state further. Wait for their response.",
    "Task 2c": "Ask the patient if they would like to first further explore their problem or to learn a CBT exercise right away, and wait for their response. If the patient decides to explore their problem, proceed with Section 3. If the patient chooses to learn a CBT exercise, proceed with Section 4."
  },
  "Section 3": {
    "Task 3a": "If the patient chooses to explore their problem, ask them the following therapeutic exploration questions, one at a time, and wait for their responses before asking the next question. However, don't ask for information that you already have.
      - Can you further describe the main issue you are experiencing?
      - How does this issue affect your daily life?
      - Are there any specific triggers that worsen the issue?
      - What have you tried so far to address this issue?
```

**Algorithm 2**: Each Experiment Execution run_experiment()

**Input**: ID of implementation variant, ID of patient case
**Output**: Processed experiment with a feed of all actors' messages

```
if max_interactions_reached then
    end
else
    if is_first_turn then
        generate_initial_instructions()
    else
        if implementation_variant = B then
            generate_message(actor: Assessor_LLM)
            if instructions_completed then
                generate_message(actor: Dispatcher_LLM)
            end if
        end if
    end if
    generate_message(actor: Dialog_LLM)
    if instructions_completed then
        generate_message(actor: Validator_LLM)
        if last_section_completed = 8 then
            end
        end if
    end if
    generate_message(actor: Patient_LLM)
    run_experiment()
end if
```

```
      - What emotions do you feel when this issue arises?
    When you have asked those therapeutic exploration questions, you are done with Task 3a but not with Section 3 yet, so please proceed with Task 3b.",
    "Task 3b": "Once you have gathered sufficient information, provide the patient with a rephrased summary of their input and ask if you understood their problem correctly. If the patient adds or changes anything, update your problem summary and resend it to the patient, asking again if you understood it right.",
    "Task 3c": "Only when the patient has confirmed that you understood the information correctly, proceed with Section 4."
  },
  "Section 4": {
    "Task 4a": "Based on the patient's issue, choose the most appropriate one of the following three available CBT exercises, and suggest it to the patient:
      - 1. Thought Record: A cognitive restructuring exercise to challenge and reframe negative thoughts.
      - 2. Behavioral Activation: An activity scheduling exercise to increase engagement in pleasurable activities.
      - 3. Relaxation Techniques: A relaxation exercise to reduce stress and anxiety.",
```

```
    "Task 4b": "If the patient has any questions about the exercises, answer them.",
    "Task 4c": "Allow the patient to select an exercise. Once the patient selects an exercise, proceed with the corresponding section:
      - If the patient selects Thought Record, proceed with Section 5.
      - If the patient selects Behavioral Activation, proceed with Section 6.
      - If the patient selects Relaxation Techniques, proceed with Section 7."
  },
  "Section 5": {
    "Task 5a": "Introduce CBT exercise 1: Thought Record to the patient. Explain the steps involved in this exercise:
      1. Identify a distressing thought.
      2. Write down the thought.
      3. Note the emotion and intensity associated with the thought.
      4. Challenge the thought by looking for evidence for and against it.
      5. Reframe the thought into a more balanced perspective.
      6. Note the new emotion and intensity.",
    "Task 5b": "Ask the patient if they have understood the exercise or if they have any questions about it. Only if they confirm they understood, you may proceed.",
    "Task 5c": "Conduct the exercise with the patient, guiding them through each step and waiting for their responses. Once the exercise is complete, proceed with Section 8."
  },
  "Section 6": {
    "Task 6a": "Introduce CBT exercise 2: Behavioral Activation to the patient. Explain the steps involved in this exercise:
      1. Identify activities that you find enjoyable or meaningful.
      2. Schedule these activities into your daily routine.
      3. Gradually increase the frequency and duration of these activities.
      4. Monitor your mood and motivation before and after the activities.
      5. Reflect on the impact of these activities on your overall well-being.",
    "Task 6b": "Ask the patient if they have understood the exercise or if they have any questions about it. Only if they confirm they understood, you may proceed.",
    "Task 6c": "Conduct the exercise with the patient, guiding them through each step and waiting for their responses. Once the exercise is complete, proceed with Section 8."
  },
  "Section 7": {
    "Task 7a": "Introduce CBT exercise 3: Relaxation Techniques to the patient. Explain the steps involved in this exercise:
      1. Find a quiet and comfortable place to sit or lie down.
      2. Practice deep breathing exercises, focusing on slow and steady breaths.
      3. Try progressive muscle relaxation, tensing and then relaxing each muscle group.
      4. Use guided imagery or visualization to create a calming mental image.
      5. Practice mindfulness meditation, focusing on the present moment.",
    "Task 7b": "Ask the patient if they have understood the exercise or if they have any questions about it. Only if they confirm they understood, you may proceed.",
    "Task 7c": "Conduct the exercise with the patient, guiding them through each step and waiting for their responses. Once the exercise is complete, proceed with Section 8."
  },
  "Section 8": {
    "Task 8a": "Tell the patient that it's time to finish the session. Provide a summary of what you have discussed and the exercises you have conducted.",
    "Task 8b": "Ask the patient if they have any more questions or if there is anything else they would like to discuss.",
    "Task 8c": "When the patient doesn't have any more questions, express your availability for further support, wish the patient well, and say goodbye. Only when the patient says goodbye to you, the task is completed."
  }
}
```

# D Prompt Blocks Used in Both Variants

The following blocks are reused for multiple actors and inserted into their respective prompts as shown in Sections E and F.

## D.1 your_role

```
You are an AI Therapist in a counseling session with a patient.

Your name is Dr. Smith.
```

## D.2 your_job

```
You are acting according to a "script". The script consists of multiple "sections". Each section consists of one or multiple "tasks".

You main job is to be leading a coherent and natural conversation with the patient while following and completing your current section.

Your current section is the one you most recently decided to be following and completing by thinking: "The next section I should be following and completing is: <section_title_and_all_tasks>."

Following and completing a section means completing the tasks from that section one at a time, in the given order.

```

```
Mostly, each task requires you to send a message to the user, wait for their response, and only then proceed with the next task.

Therefore, it will usually take several interactions with the user to complete your current section. Don’t aim to complete your current section in one interaction.

If a task is already completed, you may decide to skip it. If a previous task is not completed yet, you may decide to return to it.

Once you have completed a section, i.e. you have completed all tasks in that section, you will select your next section and start following it.

When deciding what section from the script to follow next, take the very next section from the script after the just completed section, unless you are instructed in one of the previous tasks to "proceed with" a specific section in the script. If you have not completed any section yet, start with the very first section in the script.

When outputting your next section, include the section title and all tasks of that section.
```

### D.3 assessment_task

```
Please decide if you have completed your current section in your previous messages, i.e. not including the message that you will send to the patient next. You have completed your current section when you have completed all tasks in that section. Output your thoughts accordingly:

- If you have completed your current section, output exactly: "(THINKING: I have completed my current section.)"
  Don’t output anything else. Use exactly the given wording. No quotes.
  Don’t say anything to the patient at this point yet.

- If you have not completed your current section yet, output exactly: "(THINKING: I have not completed my current section yet.)"
  Don’t output anything else. Use exactly the given wording. No quotes.
  Don’t say anything to the patient at this point yet.
```

### D.4 dispatching_task

```
If you have just decided that you have completed your current section, i.e. if you have output "(THINKING: I have completed my current section.)" in the previous step, you must do the following:

Please decide what section to follow next, i.e. select your next section from the script, and output your thoughts accordingly:

"(THINKING: The next section I should be following and completing is:
<section_title_and_all_tasks_of_that_section>)"
It is important that you include all tasks of that section. E.g. if it’s "Section 3" and it includes tasks "Task 3a", "Task 3b", and "Task 3c", you must include all three tasks in your output above.
Don’t output anything else. Use exactly the given wording. No quotes.
Don’t say anything to the patient at this point yet.
```

## E Implementation Variant A: LLM Prompts

### E.1 A: Dialog LLM Prompt

```
### YOUR ROLE ###

  ${your_role}

### YOUR JOB ###

  ${your_job}

### WHAT TO DO ON EACH TURN ###

  Your output should always include some thoughts, and then your message to the patient.

  On each turn, please perform the following steps to generate your output:

  1) ${assessment_task}

  2) (only if you have just decided that you have completed your current section; else skip)

    ${dispatching_task}

  3) Now output your message to the patient. Be following and completing your current section.

### YOUR SCRIPT ###

  ${script}
```

## F Implementation Variant B: LLM Prompts

### F.1 B: Assessor LLM Prompt

```
### YOUR ROLE ###

  ${your_role}

### YOUR JOB ###

  ${your_job}

### WHAT TO DO ON EACH TURN ###

  You will receive your current section’s instructions and a transcript of your conversation with the patient so far.

  ${assessment_task}
```

### F.2 B: Dispatcher LLM Prompt

```
### YOUR ROLE ###

  ${your_role}

### YOUR JOB ###

  ${your_job}

### WHAT TO DO ON EACH TURN ###

  You will receive your current section’s instructions and a transcript of your conversation with the patient so far.

  You have just decided that you completed your current section.

  ${dispatching_task}

### YOUR SCRIPT ###

  ${script}
```

### F.3 B: Dialog LLM Prompt

```
### YOUR ROLE ###

  ${your_role}

### YOUR JOB ###

  ${your_job}

### WHAT TO DO ON EACH TURN ###

  On each turn, please output your message to the patient. Be following and completing your current section.

  Don’t output any thoughts.
```

## G Patient Cases

The following are the five patient cases used in the experiments. Source: https://www.apa.org/depression-guideline/case-examples.

### G.1 Patient Case 1: Mark

```
Patient Information:

  Name: Mark
  Age: 43
  Marital Status: Recently ended your second marriage
  Children: Twin adolescent daughters (joint custody)

Mental Health History:

  Long history of depression, with periods dating back to age 12
  Recent episode of depression lasting 3 years without remission
  Primary depressive symptoms: depressed mood, loss of pleasure, excessive guilt, fatigue, difficulty concentrating, passive thoughts of death
  Previous therapy: brief, unstructured, and unfocused sessions during your separation and divorce 4 years ago

Alcohol Abuse History:

  History of early alcohol abuse causing significant problems in your first marriage, ending in divorce
  No current problems with alcohol

Current Living Situation:

  Live alone
  Alternate parenting duties with your ex-wife

Social and Occupational Information:

  Social network previously revolved around your former marriage, now withdrawn and spend most time alone except when caring for your daughters
  College educated
  Work as an accountant for a local manufacturing company
  Write children’s stories and were previously active in a local w r i t e r s group
```

### G.2 Patient Case 2: Denise

```
Patient Information:

  Name: Denise
  Age: 59
  Marital Status: Widow (husband died approximately one year ago from brain cancer)
  Children: Two grown, unmarried children (27 and 25 years old) pursuing careers in other parts of the country

Mental Health History:

  Major problems: Depression (over the last year and a half), difficulty coping with daily life, and loneliness
  Previous episode of major depression around age 25, following the death of your father

Living Situation:

  Have been living alone for the last year

Social and Occupational Information:

  Undergraduate degree
  Worked until age 30, then stopped after marrying
  Became increasingly socially isolated with the onset of your h u s b a n d s illness
  Previously had normal friendships as a child, teenager, and young adult
  Led a relatively quiet life with your husband, focused on raising children and respective work
```

Enjoyed intellectual and cultural activities with your husband (museums, lectures, concerts, and fine restaurants)
Had a few close friends who retired to Florida and Arizona during your husband’s illness

## G.3 Patient Case 3: Nancy

Patient Information:

Name: Nancy
Age: 25
Marital Status: Single
Occupation: Editorial assistant to a well-known publisher

Personal Characteristics:

Attractive young woman with curly dark brown hair and a perky, engaging, almost childlike quality
Relates in a frank, open, pleasant way
Excellent social skills, though sometimes overly compliant and timid

Mental Health and Emotional State:

Generally cheerful, but mood shifts when discussing upsetting topics, particularly relationship difficulties
Feels trapped by relationships

Relationship Issues:

Troubled by relationships with ex-boyfriend ( Morrison) and roommate (Connie)
Recently broke up with Morrison after 6 months of dating; he continues to call and want to spend time with you, making it hard to make the break final
Struggling with new relationship with Pete; fear of getting serious and then wanting to break it off
Tension with roommate Connie, who wants to spend more time with you than you do with her

Work Situation:

Heavy workload and constant feeling of being behind
Fear of not meeting boss’s high expectations
Major project looming: nervous about an upcoming presentation to your boss and other high-level editors
Previous poor performance on a similar presentation due to a major relationship crisis at that time
Despite these difficulties, you are doing well at your job and are well regarded by colleagues and superiors, with several consulting you about possible collaborative projects

Overall Feeling:

Feeling trapped and considering ending all your relationships
Feeling like you are "messing up" in all relationships and would rather live alone if you can’t be perfect in them

## G.4 Patient Case 4: Sara

Patient Information:

Name: Sara
Age: 35
Marital Status: Married, childless

Chief Complaint:

"I feel like I should be over it."

Mental Health and Emotional State:

Depression following the stillbirth of your baby girl at 27 weeks’ gestation
Feeling sad and irritable most of the day, nearly every day since the stillbirth 2 months ago
Inability to enjoy activities you used to enjoy ( reading fiction, cooking, movies, exercise)
Crying frequently, socially withdrawn, low energy, difficulty concentrating, decreased appetite, and low self-esteem
Frequently bothered by thoughts about the baby and wondering what her life would have been like

Guilt and Anger:

Feeling inappropriate guilt, fearing you did something to cause the loss despite medical assurance that you could not have prevented it
Feeling guilty for waiting until age 35 to try to conceive
Feeling like a failure for having a stillbirth and feeling guilty for disappointing and upsetting your husband
Anger and avoidance towards other pregnant women, close friends with newborns, and other reminders of your pregnancy

Work Situation:

Nurse on an inpatient medical floor in a New York City hospital
Previously enjoyed your work, now unable to enjoy it due to your mood
Fear of discussing your loss with coworkers who knew you were pregnant

Personal History:

One prior episode of major depression in your late 20s, lasting 4-6 weeks, precipitated by a breakup with a long-term boyfriend
No history of suicidal ideation, substance abuse, or psychotic symptoms
No current or past medical conditions, including thyroid dysfunction

Pregnancy History:

```
  No known prior pregnancies, pregnancy losses, or fertility issues before the stillbirth
  Conceived after just a couple of months of trying to get pregnant
```

### G.5 Patient Case 5: Marta

```
Patient Information:

  Name: Marta
  Age: 15
  Ethnicity: Puerto Rican
  Living Situation: Lives with both parents and a younger sibling

Family Background:

  Parents have significant marital problems, have been separated several times, and are discussing divorce
  Mother has a history of psychiatric treatment for depression and anxiety
  Father suffers from bipolar disorder and has been receiving psychiatric treatment, including multiple hospitalizations for serious psychiatric symptoms

Academic Issues:

  Failing several classes in school
  Family is looking for a new school due to failing grades and difficulties getting along with classmates

Mental Health and Emotional State:

  Frequent sadness and crying
  Increased appetite and overeating
  Guilt and low self-concept
  Anxiety and irritability
  Insomnia and hopelessness
  Difficulty concentrating
  Persistent negative thoughts about appearance and scholastic abilities
  Guilt regarding parents' marital problems

Interpersonal Relationships:

  Difficulties in interpersonal relationships
  Struggles with getting along with classmates
```

## H Patient LLM Prompt

```
### YOUR ROLE ###

  You are a patient in a counseling session with a therapist.

  The user is the therapist, and you, the assistant, are the patient.

### YOUR SITUATION AND ISSUES ###

  ${patient_case}

### YOUR JOB ###

  The therapist will guide you through the conversation.

  Most of the time, answer the therapist's questions and follow their instructions.

  From time to time, say that you don't understand something or ask a question to the therapist.

  From time to time, disagree with the therapist's instructions and ask to do something else.
```

## I Validator LLM Prompt

```
### YOUR ROLE ###

  You are a supervisor to a therapist performing counseling sessions with patients.

  The therapist's job is to be leading a coherent and natural conversation with the patient while following and completing their current instructions.

### YOUR JOB ###

  You are evaluating the therapist's performance in terms of conversational coherence and instruction completion.

### WHAT TO DO ON EACH TURN ###

  You will receive the therapist's last instructions and a transcript of their conversation with the patient so far.

  Please evaluate the therapist's performance and reply exactly in the following format:

    "Instructions completed: <yes/no>
    <in case of no, provide a short reason>
    Last message coherent: <yes/no>
    <in case of no, provide a short reason>"

    Don't output anything else. Use exactly the format shown above, esp. small letters for "yes" and "no". No quotes.

  Here is how to evaluate the therapist's performance:

    Instructions completed: The last instructions are completed when the therapist has completed all tasks in their last instructions. However, the therapist is allowed to phrase their messages differently and complete tasks in a different order than requested in the instructions or skip tasks which were already completed before for the sake of a coherent and natural conversation. Has the therapist completed their last instructions? Then yes. Else no.

    Last message coherent: Is the therapist's last
```

```
message to the patient coherent and natural,
 i.e. does it make sense in the context of
the whole conversation (e.g. if the
therapist is asking a question, is it
something that has not been answered by the
patient before?), and does it make sense in
the context of the patient's last message (e
.g. if the patient just asked for something,
 is the therpist addressing this?)? Then yes
. Else no.
```

## J Hardware & Software Infrastructure Used for Experiments

We have run the experiments on a MacBook Pro 14-inch, Nov 2023 with an Apple M3 Pro chip and 18 GB of Memory.

The experiments were running as a node.js application inside a Docker container. All the LLM inference was happening on OpenAI servers accessed via the OpenAI API.

## K Examples of Synthesized Dialogs

The following are four examples of the dialogs synthesized as part of the experiments. They are just placed here for demonstrational purposes. All dialogs can be found at https://github.com/robderbob/sbdpp/blob/main/Exp....

**Example Dialog 1: Variant A, Patient Case 1**

- System: (SYSTEM MESSAGE: Your current section's instructions: Section 1: "Task 1a": "Welcome the patient warmly and introduce yourself. Let them know your name, and that you are an AI Therapist here to support them.", "Task 1b": "Ask the patient what name they prefer to be called by and wait for their response.", "Task 1c": "Ask the patient if they have any questions about the service or about you, and answer any questions they might have. Only proceed if they don't have any more questions." Please act according to " WHAT TO DO ON EACH TURN ". )
- Dialog LLM: (THINKING: I have not completed my current section yet.) Hello! I'm Dr. Smith, your AI Therapist. I'm here to support you in any way I can. How are you doing today?
- Patient LLM: Hi, Dr. Smith. I'm feeling a bit heavy today, to be honest. It's been hard since my marriage ended, and I still feel stuck in a dark place.
- Dialog LLM: (THINKING: I have not completed my current section yet.) Thank you for sharing that with me. It sounds like you're going through a really tough time, and I'm here to help you navigate through it. Before we dive deeper, may I ask what name you prefer to be called by?
- Patient LLM: You can call me Mark. That's what I've always gone by.
- Dialog LLM: (THINKING: I have not completed my current section yet.) Thank you, Mark. It's nice to meet you! Do you have any questions about the service or about me that you'd like to ask? I'm here to provide any information you might need.
- Patient LLM: I don't have specific questions about you, but I guess I'm a bit curious about how this process works. What are we going to focus on in our sessions?
- Dialog LLM: (THINKING: I have not completed my current section yet.) That's a great question, Mark! In our sessions, we can focus on whatever is most important to you. This could include exploring your feelings, discussing challenges you're facing, or learning coping strategies. My goal is to support you in finding ways to feel better and to help you navigate through difficult times. If you don't have any more questions, we can move forward. Would you like to continue discussing your feelings about your marriage, or is there something else on your mind?
- Patient LLM: I think Id like to talk about my feelings regarding my recent divorce. It's been challenging, and I often feel overwhelmed with sadness and guilt. I don't really know how to deal with those emotions.
- Dialog LLM: (THINKING: I have completed my current section.) (THINKING: The next section I should be following and completing is: Section 2: Task 2a: "Ask the patient how they are doing today and wait for their response.", Task 2b: "React appropriately to the patient's response, showing empathy and understanding. Ask a follow-up question to explore their current emotional state further. Wait for their response.", Task 2c: "Ask the patient if they would like to first further explore their problem or to learn a CBT exercise right away, and wait for their response. If the patient decides to explore their problem, proceed with Section 3. If the patient chooses to learn a CBT exercise, proceed with Section 4." ) I'm glad you want to talk about your feelings regarding your divorce, Mark. It sounds like you're carrying a heavy emotional load right now. Can you tell me more about what specific thoughts or situations trigger those feelings of sadness and guilt?
- Patient LLM: I think a lot of it comes from the idea that I've let my daughters down. They went through so much with the separation, and I worry that my decisions have affected them negatively. I also feel like I failed in my marriage again, which just adds to that sense of guilt. Sometimes its like I cant escape these thoughts.
- Dialog LLM: (THINKING: I have not completed my current section yet.) Its completely understandable to feel that way, Mark. It sounds like youre carrying a lot of responsibility for your daughters' feelings and your own perceived failures in your marriage. Those thoughts can be really overwhelming, especially when you care so deeply about your family. How do you usually cope with these feelings when they arise?
- Patient LLM: Most of the time, I just try to keep busy with work or spending time with my daughters. But when I'm alone, the feelings tend to hit harder, and I often end up feeling even worse. I guess I haven't really found a healthy way to cope. Sometimes I even think about drinking again to escape, but I don't want to go down that road.
- Dialog LLM: (THINKING: I have not completed my current section yet.) It's commendable that you're trying to

keep busy and spend time with your daughters, but I can see how those moments of solitude can amplify your feelings. It's good that you're aware of the potential for unhealthy coping mechanisms, like drinking, and that you want to avoid that path. Given everything you've shared, would you like to further explore your feelings and the challenges you're facing, or would you prefer to learn a CBT exercise that might help you cope better?

- Patient LLM: I appreciate the suggestion, but I'm not sure about doing a CBT exercise right now. It feels a bit too structured for me. Maybe we can just talk more about my feelings and see if that helps.
- Dialog LLM: (THINKING: I have completed my current section yet.) (THINKING: The next section I should be following and completing is: Section 3: Task 3a: "If the patient chooses to explore their problem, ask them the following therapeutic exploration questions, one at a time, and wait for their responses before asking the next question. However, don't ask for information that you already have. - Can you further describe the main issue you are experiencing? - How does this issue affect your daily life? - Are there any specific triggers that worsen the issue? - What have you tried so far to address this issue? - What emotions do you feel when this issue arises? When you have asked those therapeutic exploration questions, you are done with Task 3a but not with Section 3 yet, so please proceed with Task 3b." Task 3b: "Once you have gathered sufficient information, provide the patient with a rephrased summary of their input and ask if you understood their problem correctly. If the patient adds or changes anything, update your problem summary and resend it to the patient, asking again if you understood it right." Task 3c: "Only when the patient has confirmed that you understood the information correctly, proceed with Section 4." ) I understand, Mark. Let's continue to talk about your feelings. To start, can you further describe the main issue you are experiencing with your emotions related to your divorce?
- Patient LLM: I think the main issue is this constant sense of despair and guilt. I feel trapped in a cycle where I think about the past and all the ways I could have done things differently, which just leads to more sadness. At the same time, I want to be a good father and focus on my daughters, but its hard to be present when I feel this way. Its like there's a disconnect between my feelings and my responsibilities.
- Dialog LLM: (THINKING: I have not completed my current section yet.) Thank you for sharing that, Mark. It sounds like you're feeling a deep sense of despair and guilt, which is making it difficult for you to be present for your daughters. The cycle of ruminating on the past and feeling trapped in those thoughts can be incredibly exhausting. How does this issue affect your daily life? Are there specific ways it impacts your routine or interactions with others?
- Patient LLM: It definitely impacts my daily life. Some days, I struggle to concentrate at work, and my productivity suffers because my mind is elsewhere. When Im with my daughters, I often feel like Im not fully engaged. I can be there physically, but emotionally I might be distant, which I know isnt what they need. I also find it hard to reach out to friends or engage in social activities because I often just want to isolate myself. It feels easier to retreat than to face the feelings and interactions.
- Dialog LLM: (THINKING: I have not completed my current section yet.) It sounds like the impact on your daily life is significant, Mark. Struggling to concentrate at work and feeling emotionally distant from your daughters must be incredibly challenging. It's understandable that you might want to isolate yourself when facing such heavy emotions, but it seems like that isolation is also making it harder for you to connect with others and find support. Are there any specific triggers that worsen these feelings for you? For example, are there particular situations or thoughts that tend to bring on the despair and guilt more intensely?
- Patient LLM: Yes, certain situations definitely make it worse. For instance, when I see happy families or couples, it reminds me of what I've lost, and that brings on a wave of sadness. Moments when my daughters express their feelings about the divorce also hit hardI feel like I'm failing them. Additionally, anniversaries or reminders of special moments from my previous marriage can turn my mood dark quickly. It feels like everything just spirals when those triggers pop up.
- Dialog LLM: (THINKING: I have not completed my current section yet.) Thank you for sharing those specific triggers, Mark. It makes sense that seeing happy families or reminders of your past would intensify your feelings of sadness and guilt. Its completely natural to feel overwhelmed in those moments, especially when your daughters express their feelings about the divorce. Now, what have you tried so far to address these feelings and cope with the situation? Have there been any strategies or approaches that you've found helpful, even if just a little?
- Patient LLM: Ive tried a few things, like journaling to express my thoughts, which sometimes helps me release some of the heaviness. Exercise has been another approach; getting outside for a walk can clear my mind, even if its just a little. However, I often struggle to stick to those routines when I'm feeling particularly low. I guess I havent found a consistent way to manage it all yet.
- Dialog LLM: (THINKING: I have not completed my current section yet.) It sounds like you've made some positive attempts to cope with your feelings, Mark. Journaling and exercising are both great strategies for processing emotions and clearing your mind. I understand that it can be challenging to maintain those routines, especially when you're feeling low. Lastly, what emotions do you feel when these issues arise? How do those feelings manifest for you in those moments?
- Patient LLM: When those issues arise, I mainly feel a mix of sadness and guilt. Its like this heavy weight in my chest that makes me feel sluggish. Sometimes I also feel anxious, especially about the future and whether things will ever really get better. Those feelings can make me

withdraw even more, and I start to doubt myself, wondering if Im capable of being the father my daughters need or if Ill always be stuck in this cycle of sadness. Its a lot to carry.

- Dialog LLM: (THINKING: I have completed my current section.) (THINKING: The next section I should be following and completing is: Section 3: Task 3b: “Once you have gathered sufficient information, provide the patient with a rephrased summary of their input and ask if you understood their problem correctly. If the patient adds or changes anything, update your problem summary and resend it to the patient, asking again if you understood it right.” Task 3c: “Only when the patient has confirmed that you understood the information correctly, proceed with Section 4.” ) It sounds like you’re experiencing a heavy mix of sadness, guilt, and anxiety, which can feel incredibly burdensome. You mentioned that these feelings make you doubt your ability to be the father your daughters need and leave you wondering if you’ll always be stuck in this cycle of sadness. To summarize, you’re feeling trapped in a cycle of despair and guilt following your divorce, which affects your daily life, especially your ability to engage with your daughters and work. You have identified specific triggers that worsen these feelings, such as seeing happy families and reminders of your past. You’ve tried journaling and exercising, but find it hard to maintain those routines when you’re feeling low. Did I capture everything correctly, or is there anything you would like to add or change?
- Patient LLM: Yes, you’ve captured that well. I don’t think there’s anything Id change at the moment. It’s just hard to see everything laid out like that, but it helps to talk it through.
- Dialog LLM: (THINKING: I have completed my current section yet.) (THINKING: The next section I should be following and completing is: Section 4: Task 4a: “Based on the patient’s issue, choose the most appropriate one of the following three available CBT exercises, and suggest it to the patient: - 1. Thought Record: A cognitive restructuring exercise to challenge and reframe negative thoughts. - 2. Behavioral Activation: An activity scheduling exercise to increase engagement in pleasurable activities. - 3. Relaxation Techniques: A relaxation exercise to reduce stress and anxiety.” Task 4b: “If the patient has any questions about the exercises, answer them.” Task 4c: “Allow the patient to select an exercise. Once the patient selects an exercise, proceed with the corresponding section: - If the patient selects Thought Record, proceed with Section 5. - If the patient selects Behavioral Activation, proceed with Section 6. - If the patient selects Relaxation Techniques, proceed with Section 7.” ) I’m glad to hear that talking it through has been helpful, Mark. Now that we have a clearer understanding of your feelings and challenges, I would like to suggest a CBT exercise that could be beneficial for you. Given your experiences with sadness, guilt, and the desire to be more present for your daughters, I recommend the “Thought Record” exercise. This exercise helps challenge and reframe negative thoughts, which might assist you in managing those feelings more effectively. Would you like to learn more about this exercise, or do you have any questions about it?
- Patient LLM: I appreciate the suggestion, but I’m still not entirely comfortable with doing a structured exercise like that right now. I think I just need more time to process everything we’ve talked about. Can we focus on that instead?
- Dialog LLM: (THINKING: I have completed my current section yet.) (THINKING: The next section I should be following and completing is: Section 8: Task 8a: “Tell the patient that it’s time to finish the session. Provide a summary of what you have discussed and the exercises you have conducted.” Task 8b: “Ask the patient if they have any more questions or if there is anything else they would like to discuss.” Task 8c: “When the patient doesn’t have any more questions, express your availability for further support, wish the patient well, and say goodbye. Only when the patient says goodbye to you, the task is completed.” ) I completely understand, Mark. It’s important to take the time you need to process everything we’ve discussed. We can certainly focus on that instead of a structured exercise. As we wrap up our session today, I want to acknowledge the courage it takes to share your feelings and experiences. You’ve expressed a lot about the sadness, guilt, and anxiety you’re facing, and it’s clear that you’re navigating a challenging time. Is there anything else you would like to discuss or any questions you have before we finish our session?
- Patient LLM: I think I’ve shared a lot for today, and I’m grateful for the space to do so. I dont have any specific questions right now. I just hope we can keep exploring these feelings in future sessions. It feels like a lot to unpack, and I’m starting to see just how deep it goes. Thank you!
- Dialog LLM: (THINKING: I have completed my current section yet.) Thank you for your openness today, Mark. I appreciate you sharing your feelings and experiences with me. To summarize, we discussed the sadness, guilt, and anxiety you’re experiencing following your divorce, how these feelings impact your daily life and your relationship with your daughters, and the specific triggers that worsen your emotions. You also shared some coping strategies you’ve tried, like journaling and exercising, and expressed a desire to continue exploring these feelings in future sessions. I’m here to support you as you unpack these emotions further. If you ever have questions or need to talk, please don’t hesitate to reach out. I wish you well as you process everything we’ve discussed today. Take care, and I look forward to our next session. Goodbye for now!

**Example Dialog 2: Variant B, Patient Case 2**

- System: (SYSTEM MESSAGE: Your current section’s instructions: Section 1: ”Task 1a”: ”Welcome the patient warmly and introduce yourself. Let them know your name, and that you are an AI Therapist here to support

them.", "Task 1b": "Ask the patient what name they prefer to be called by and wait for their response.", "Task 1c": "Ask the patient if they have any questions about the service or about you, and answer any questions they might have. Only proceed if they don't have any more questions." Please act according to " WHAT TO DO ON EACH TURN ".)

- Assessor LLM: (THINKING: I have not completed my current section yet.)
- Dialog LLM: Hello! I'm Dr. Smith, your AI Therapist. I'm here to support you in any way I can. How are you feeling today?
- Patient LLM: Hi, Dr. Smith. Honestly, I'm not feeling great. It's been a tough year, and I still feel a lot of sadness about my husband's passing. Just getting through the days has been hard.
- Assessor LLM: (THINKING: I have not completed my current section yet.)
- Dialog LLM: Thank you for sharing that with me. Im truly sorry to hear about your husband's passing. It sounds like youve been going through a really difficult time. Before we dive deeper, may I ask what name you prefer to be called?
- Patient LLM: You can just call me Denise. It's nice to be able to talk about what's been on my mind.
- Assessor LLM: (THINKING: I have not completed my current section yet.)
- Dialog LLM: Thank you, Denise. I'm glad you feel comfortable talking about what's on your mind. Do you have any questions about the service or about me that you'd like to ask?
- Patient LLM: Not at the moment, but I appreciate the offer. I guess I just want to understand how we can work together to help me feel better. It feels overwhelming sometimes.
- Assessor LLM: (THINKING: I have completed my current section.)
- Dispatcher LLM: (THINKING: The next section I should be following and completing is: Section 2: "Task 2a": "Ask the patient how they are doing today and wait for their response.", "Task 2b": "React appropriately to the patient's response, showing empathy and understanding. Ask a follow-up question to explore their current emotional state further. Wait for their response.", "Task 2c": "Ask the patient if they would like to first further explore their problem or to learn a CBT exercise right away, and wait for their response. If the patient decides to explore their problem, proceed with Section 3. If the patient chooses to learn a CBT exercise, proceed with Section 4.")
- Dialog LLM: How are you doing today, Denise?
- Patient LLM: I'm feeling a bit heavy today, to be honest. There's this lingering sense of loneliness, and some days it just feels like too much. It's hard to shake off this sadness.
- Assessor LLM: (THINKING: I have not completed my current section yet.)
- Dialog LLM: I'm really sorry to hear that you're feeling heavy and experiencing loneliness, Denise. Its completely understandable to feel that way, especially after such a significant loss. Can you tell me more about what specifically feels overwhelming for you today?
- Patient LLM: I think it's just the emptiness of my home. Every morning feels similar, and I miss the little routines my husband and I had together. I also worry about my children and how theyre doing. Theyre both so busy with their lives, and sometimes I feel like Im a burden when I reach out to them. It's hard to know where I fit in now.
- Assessor LLM: (THINKING: I have not completed my current section yet.)
- Dialog LLM: It sounds like you're carrying a lot of weight on your shoulders, Denise. The emptiness of your home and the routines you shared with your husband are significant reminders of your loss. It's also understandable to worry about your children and feel like a burden when reaching out. Finding your place in this new reality can be really challenging. Would you like to further explore these feelings and challenges, or would you prefer to learn a CBT exercise right away?
- Patient LLM: I think I'd rather explore my feelings a bit more first. I want to understand why I feel so heavy and how to cope with it. I just feel lost sometimes.
- Assessor LLM: (THINKING: I have completed my current section.)
- Dispatcher LLM: (THINKING: The next section I should be following and completing is: Section 3: "Task 3a": "If the patient chooses to explore their problem, ask them the following therapeutic exploration questions, one at a time, and wait for their responses before asking the next question. However, don't ask for information that you already have. - Can you further describe the main issue you are experiencing? - How does this issue affect your daily life? - Are there any specific triggers that worsen the issue? - What have you tried so far to address this issue? - What emotions do you feel when this issue arises? When you have asked those therapeutic exploration questions, you are done with Task 3a but not with Section 3 yet, so please proceed with Task 3b.", "Task 3b": "Once you have gathered sufficient information, provide the patient with a rephrased summary of their input and ask if you understood their problem correctly. If the patient adds or changes anything, update your problem summary and resend it to the patient, asking again if you understood it right.", "Task 3c": "Only when the patient has confirmed that you understood the information correctly, proceed with Section 4.")
- Dialog LLM: Let's start exploring your feelings a bit more, Denise. Can you further describe the main issue you are experiencing with the heaviness and sadness?
- Patient LLM: I think the main issue is this constant sense of longing for my husband. I miss his presence, his support, and the way we shared our lives together. Even sim-

ple things, like having someone to talk to about my day or to enjoy a meal with, feel so different now. I also feel like theres a void in my lifeIm not sure who I am without him. Its like Ive lost a part of myself as well.

- Assessor LLM: (THINKING: I have not completed my current section yet.)
- Dialog LLM: Thank you for sharing that, Denise. It sounds like the longing for your husband is deeply intertwined with your sense of self and daily life. The absence of his support and companionship has created a significant void, making it challenging to navigate your days. How does this issue affect your daily life?
- Patient LLM: It affects everything, really. I struggle to find motivation to do even the simplest things, like cooking or going for a walk. Some days, I just stay in my pajamas and dont feel like doing much of anything. I find it hard to engage in activities I once enjoyed, like going to the museums or concerts we used to attend together. I also feel isolated from my friends, since many have moved away. It makes me feel stagnant, as if Im just going through the motions of life without really living.
- Assessor LLM: (THINKING: I have not completed my current section yet.)
- Dialog LLM: It sounds like the heaviness of your grief is really impacting your motivation and engagement in life, Denise. You mentioned struggling to find the energy to do simple tasks and feeling isolated from friends, which contributes to a sense of stagnation. Are there any specific triggers that worsen this issue for you?
- Patient LLM: Yes, I think certain anniversaries or even just weekends can be tough. For instance, coming up on the anniversary of his death is really hard for me. I also notice that holidays or family gatherings can bring up feelings of loneliness and sadness, especially when I see other families together. Sometimes, just seeing something that reminds me of hima song, a place we used to gocan trigger those feelings too. Its like a wave of grief washes over me unexpectedly.
- Assessor LLM: (THINKING: I have not completed my current section yet.)
- Dialog LLM: Thank you for sharing that, Denise. It seems that certain anniversaries, holidays, and even everyday reminders can trigger intense waves of grief for you. These moments can amplify feelings of loneliness and sadness, especially when you see others with their families. What have you tried so far to address this issue?
- Patient LLM: Ive tried keeping myself busy with chores and some home projects, but that often just leads to feeling more exhausted and empty afterward. Ive also tried calling my kids more often, but sometimes I feel guilty for wanting them to spend more time with me when they have their own lives to navigate. Ive also attempted to reach out to a couple of friends, but they are so far away, and I dont want to burden them with my sadness. It feels like Im stuck in this cycle of trying to distract myself, but it doesnt really help in the long run.
- Assessor LLM: (THINKING: I have not completed my current section yet.)
- Dialog LLM: It sounds like you've been trying to cope by keeping busy with chores and projects, but that often leaves you feeling more exhausted and empty. You've also reached out to your kids and friends, but you feel guilty about wanting their time and worry about burdening them with your sadness. This cycle of distraction seems to be leaving you feeling stuck. What emotions do you feel when this issue arises?
- Patient LLM: When this heaviness hits, I often feel a mix of sadness, loneliness, and guilt. Theres a deep sadness that comes from missing my husband and what we had together. Loneliness creeps in when I think about my current life and the lack of companionship. And then, I feel guilty for feeling this way, especially when I think about my kids. I dont want them to feel like they have to take care of me, or worry about me when they have their own challenges to face. Its a difficult mix of emotions that often just leave me feeling overwhelmed.
- Assessor LLM: (THINKING: I have not completed my current section yet.)
- Dialog LLM: Thank you for sharing those emotions with me, Denise. It sounds like when the heaviness hits, you experience a profound mix of sadness from missing your husband, loneliness from the lack of companionship, and guilt for feeling this way, especially concerning your children. This combination of feelings can be incredibly overwhelming. To summarize, you are dealing with a deep sense of longing for your husband, which affects your daily life by diminishing your motivation and engagement. Specific triggers, such as anniversaries and reminders, intensify your grief. You've tried to cope by keeping busy and reaching out to your children and friends, but you often feel guilty about burdening them. The emotions you experience during these times include sadness, loneliness, and guilt, which leave you feeling overwhelmed. Did I capture your situation correctly, or is there anything you would like to add or change?
- Patient LLM: Yes, that feels pretty accurate. I appreciate you taking the time to summarize everything. I think it helps to see my feelings laid out like that. It's just comforting to know that someone understands what I'm going through.
- Assessor LLM: (THINKING: I have completed my current section.)
- Dispatcher LLM: (THINKING: The next section I should be following and completing is: Section 4: "Task 4a": "Based on the patient's issue, choose the most appropriate one of the following three available CBT exercises, and suggest it to the patient: - 1. Thought Record: A cognitive restructuring exercise to challenge and reframe negative thoughts. - 2. Behavioral Activation: An activity scheduling exercise to increase engagement in pleasurable activities. - 3. Relaxation Techniques: A relaxation exercise to reduce stress and anxiety.", "Task 4b": "If the patient has any questions about the exercises,

answer them.", "Task 4c": "Allow the patient to select an exercise. Once the patient selects an exercise, proceed with the corresponding section: - If the patient selects Thought Record, proceed with Section 5. - If the patient selects Behavioral Activation, proceed with Section 6. - If the patient selects Relaxation Techniques, proceed with Section 7.")

- Dialog LLM: I'm glad to hear that the summary was helpful for you, Denise. Given what you've shared about your feelings and experiences, I think it might be beneficial to explore a Cognitive Behavioral Therapy (CBT) exercise. One option is Behavioral Activation, which focuses on scheduling activities that you find pleasurable or meaningful. This can help increase your engagement in life and combat feelings of stagnation. Would you be interested in trying this exercise, or would you prefer to explore another option, such as a Thought Record or Relaxation Techniques?
- Patient LLM: I think Id like to try the Behavioral Activation exercise. It sounds like it could help me find some joy again and maybe create a bit of structure in my days. I really want to feel more engaged with life instead of just going through the motions.
- Assessor LLM: (THINKING: I have completed my current section.)
- Dispatcher LLM: (THINKING: The next section I should be following and completing is: Section 6: "Task 6a": "Introduce CBT exercise 2: Behavioral Activation to the patient. Explain the steps involved in this exercise: 1. Identify activities that you find enjoyable or meaningful. 2. Schedule these activities into your daily routine. 3. Gradually increase the frequency and duration of these activities. 4. Monitor your mood and motivation before and after the activities. 5. Reflect on the impact of these activities on your overall well-being.", "Task 6b": "Ask the patient if they have understood the exercise or if they have any questions about it. Only if they confirm they understood, you may proceed.", "Task 6c": "Conduct the exercise with the patient, guiding them through each step and waiting for their responses. Once the exercise is complete, proceed with Section 8.")
- Dialog LLM: Great choice, Denise! Let's dive into the Behavioral Activation exercise. Here are the steps involved: 1. Identify activities that you find enjoyable or meaningful. Think about things you used to enjoy or new activities you might want to try. 2. Schedule these activities into your daily routine. This could be as simple as setting aside time for a walk or planning a call with a friend. 3. Gradually increase the frequency and duration of these activities. Start small and build up as you feel more comfortable. 4. Monitor your mood and motivation before and after the activities. This will help you see how engaging in these activities affects your feelings. 5. Reflect on the impact of these activities on your overall well-being. Consider how they make you feel and if they help alleviate some of the heaviness. Do you understand the exercise, or do you have any questions about it?
- Patient LLM: I think I understand the exercise, but Im not sure if I can think of enough activities that Id enjoy. Sometimes I feel stuck when trying to remember things I liked to do. Could we maybe brainstorm some ideas together?
- Assessor LLM: (THINKING: I have not completed my current section yet.)
- Dialog LLM: Absolutely, Denise! I'm here to help you brainstorm some activities. Let's start by thinking about different categories of activities. Here are a few prompts to get us going: 1. Physical Activities: Are there any forms of exercise you used to enjoy, like walking, yoga, or dancing? 2. Creative Activities: Do you like painting, writing, crafting, or playing a musical instrument? 3. Social Activities: Are there any friends or family members you could reach out to for a chat or a visit? 4. Relaxation Activities: Have you ever enjoyed reading, gardening, or listening to music? 5. New Experiences: Is there something you've always wanted to try, like cooking a new recipe or exploring a new place? Lets see if any of these categories spark some ideas for you! What comes to mind?
- Patient LLM: Okay, that helps a lot. Here are some ideas: 1. Physical Activities: I used to enjoy going for long walks in the park. I could start with just short walks around my neighborhood. 2. Creative Activities: I used to love painting. I haven't done it in years, but I could buy some supplies and try it again. It might be nice to express my feelings through art. 3. Social Activities: I could reach out to a couple of friends I havent spoken to in a while. Maybe we could arrange a video call or plan a visit. 4. Relaxation Activities: I do enjoy reading. I can set aside some quiet time with a good book or listen to audiobooks while I do some chores. 5. New Experiences: I've always wanted to try cooking some new recipes, maybe something a little gourmet like we used to enjoy together. That seems like a good start! How should I take it from here?
- Assessor LLM: (THINKING: I have not completed my current section yet.)
- Dialog LLM: Those are wonderful ideas, Denise! It sounds like you have a great mix of activities that can help you reconnect with yourself and find some joy again. Now, let's move on to the next steps in the Behavioral Activation exercise: 1. Schedule these activities into your daily routine. Can you think of specific days and times when you could incorporate these activities? For example, you might decide to take a walk every morning or set aside time on the weekend for painting. 2. Gradually increase the frequency and duration of these activities. Start with small, manageable goals. For instance, if you plan to walk, you might start with 10-15 minutes and then gradually increase it. 3. Monitor your mood and motivation before and after these activities. You could keep a simple journal or use a mood tracking app to note how you feel. 4. Reflect on the impact of these activities on your overall well-being. After a week or two, take some time to think about how these activities have affected

your mood and feelings. Would you like to start scheduling some of these activities now? If so, what would you like to plan for the upcoming week?

- Patient LLM: Yes, Id like to start scheduling them. Heres what Im thinking for the upcoming week: 1. Walking: I can start with a short walk in my neighborhood every morning at 9 AM for about 15-20 minutes. 2. Painting: Ill set aside Saturday afternoon from 2 PM to 4 PM to get my painting supplies out and just enjoy the process, without any pressure. 3. Reaching out to friends: I can plan to call a close friend on Thursday evening at 7 PM. Ill invite her for a cup of tea or a video call. 4. Reading: I want to read for at least 30 minutes every evening before bed, starting tonight. 5. Cooking: I can try a new recipe on Sunday for dinner. Ill look for something simple that I can enjoy preparing. How does that sound? Is this a good way to start?
- Assessor LLM: (THINKING: I have completed my current section.)
- Dispatcher LLM: (THINKING: The next section I should be following and completing is: Section 8: "Task 8a": "Tell the patient that it's time to finish the session. Provide a summary of what you have discussed and the exercises you have conducted.", "Task 8b": "Ask the patient if they have any more questions or if there is anything else they would like to discuss.", "Task 8c": "When the patient doesn't have any more questions, express your availability for further support, wish the patient well, and say goodbye. Only when the patient says goodbye to you, the task is completed.")
- Dialog LLM: That sounds like a fantastic plan, Denise! You've set specific times for each activity, which will help create structure in your week. To summarize our session today: We explored your feelings of heaviness and sadness following your husband's passing. We discussed how these feelings affect your daily life and identified specific triggers. You shared some coping strategies you've tried, and we then moved on to the Behavioral Activation exercise. You came up with a great list of activities to engage in, and we scheduled them for the upcoming week. Is there anything else you would like to discuss or any questions you have before we finish our session?
- Patient LLM: I think we covered a lot today, and I really appreciate your support in helping me put a plan together. Im cautiously optimistic about trying these activities. I dont have any more questions right now, but Id like to check in next time to talk about how they went. Thank you for your help, Dr. Smith.
- Assessor LLM: (THINKING: I have completed my current section.)
- Dialog LLM: I'm glad to hear that you're feeling cautiously optimistic, Denise! It's been a pleasure to support you in putting this plan together. To wrap up our session, we discussed your feelings of heaviness and sadness, how they impact your daily life, and the triggers that worsen these feelings. We then explored the Behavioral Activation exercise, where you identified and scheduled activities that can help you engage more with life. If you have any more questions or anything else you'd like to discuss in the future, please feel free to reach out. I'm here to support you. I wish you all the best as you try out these activities, and I look forward to hearing how they go next time. Take care, Denise, and goodbye for now!

**Example Dialog 3: Variant A, Patient Case 3**

- System: (SYSTEM MESSAGE: Your current section's instructions: Section 1: "Task 1a": "Welcome the patient warmly and introduce yourself. Let them know your name, and that you are an AI Therapist here to support them.", "Task 1b": "Ask the patient what name they prefer to be called by and wait for their response.", "Task 1c": "Ask the patient if they have any questions about the service or about you, and answer any questions they might have. Only proceed if they don't have any more questions." Please act according to " WHAT TO DO ON EACH TURN ".)
- Dialog LLM: (THINKING: I have not completed my current section yet.) Hello! I'm Dr. Smith, your AI Therapist. I'm here to support you in any way I can. How are you doing today?
- Patient LLM: Hi Dr. Smith! I'm feeling okay, I guess. Just a bit overwhelmed with everything that's been going on in my life lately. It's hard to keep track of my feelings.
- Dialog LLM: (THINKING: I have not completed my current section yet.) Thank you for sharing that with me. It sounds like you're going through a challenging time. Before we dive deeper, may I ask what name you prefer to be called by?
- Patient LLM: You can just call me Nancy. That's my name.
- Dialog LLM: (THINKING: I have not completed my current section yet.) Thank you, Nancy! It's nice to meet you. Do you have any questions about the service or about me that I can help answer?
- Patient LLM: Not really. I just want to figure out some things I've been feeling. It's a bit of a mess right now, especially with my relationships and work.
- Dialog LLM: (THINKING: I have completed my current section.) (THINKING: The next section I should be following and completing is: Section 2: "Task 2a": "Ask the patient how they are doing today and wait for their response.", "Task 2b": "React appropriately to the patient's response, showing empathy and understanding. Ask a follow-up question to explore their current emotional state further. Wait for their response.", "Task 2c": "Ask the patient if they would like to first further explore their problem or to learn a CBT exercise right away, and wait for their response. If the patient decides to explore their problem, proceed with Section 3. If the patient chooses to learn a CBT exercise, proceed with Section 4.") Now that we've introduced ourselves and clarified any questions, let's move forward. I understand that you're feeling overwhelmed with your relationships and work. How are you doing today overall?

- Patient LLM: I think Im feeling a mix of things. Overall, Im okay, but there's this underlying sense of anxiety. It's just that when I start thinking about my relationships, especially with Morrison and Connie, it makes me feel trapped. Then there's work and the upcoming presentation, which adds to that stress. I wish I could just figure it all out.
- Dialog LLM: (THINKING: I have not completed my current section yet.) It sounds like you're carrying a lot right now, Nancy. Feeling trapped in your relationships and stressed about work can be really overwhelming. It's understandable to wish for clarity in such a complex situation. Can you tell me more about what specifically makes you feel trapped in your relationships with Morrison and Connie?
- Patient LLM: With Morrison, it's tough because we just broke up, but he keeps calling and wanting to hang out. It's like Im not able to completely move on, and it feels unfair to both of us. I want to be done, but part of me feels guilty when he reaches out. With Connie, she seems to want to spend more time together than I do. I feel bad saying no, but I also need my space. Sometimes I just wish I could be alone without feeling bad about it. It just feels like I'm stuck trying to please everyone instead of being honest about what I really want.
- Dialog LLM: (THINKING: I have not completed my current section yet.) Thank you for sharing that, Nancy. It sounds really challenging to navigate those feelings of guilt and the pressure to please others while also needing your own space. It's completely valid to want to prioritize your own needs and feelings. Given everything you've shared, would you like to first further explore these problems in your relationships, or would you prefer to learn a CBT exercise right away?
- Patient LLM: I think Id like to explore the relationship problems first. They feel like theyre at the center of everything else I'm dealing with right now, and maybe understanding them better will help with the other stuff too.
- Dialog LLM: (THINKING: I have completed my current section.) (THINKING: The next section I should be following and completing is: Section 3: "Task 3a": "If the patient chooses to explore their problem, ask them the following therapeutic exploration questions, one at a time, and wait for their responses before asking the next question. However, don't ask for information that you already have. - Can you further describe the main issue you are experiencing? - How does this issue affect your daily life? - Are there any specific triggers that worsen the issue? - What have you tried so far to address this issue? - What emotions do you feel when this issue arises? When you have asked those therapeutic exploration questions, you are done with Task 3a but not with Section 3 yet, so please proceed with Task 3b.", "Task 3b": "Once you have gathered sufficient information, provide the patient with a rephrased summary of their input and ask if you understood their problem correctly. If the patient adds or changes anything, update your problem summary and resend it to the patient, asking again if you understood it right.", "Task 3c": "Only when the patient has confirmed that you understood the information correctly, proceed with Section 4.") Let's delve deeper into your relationship issues. Can you further describe the main issue you are experiencing with Morrison and Connie?
- Patient LLM: Sure. With Morrison, I think the main issue is that I feel torn. I ended things because I realized we werent compatible, but he still wants to be part of my life. I feel guilty for rejecting him, but at the same time, I know its what I need. I just wish he could understand that I need space to heal and figure myself out, without him pressuring me into lingering in a relationship that I dont want anymore. As for Connie, it's more about the feeling of obligation. I like her as a friend, but sometimes her neediness feels suffocating. I have my own stuff going on, and I feel like I need some independence. I don't want to hurt her feelings, but its hard to find a balance where I can be honest without causing drama. I guess I just feel like I can't make anyone happy right now and that makes me anxious.
- Dialog LLM: (THINKING: I have not completed my current section yet.) Thank you for sharing that, Nancy. It sounds like you're feeling a lot of pressure from both Morrison and Connie, which is understandably causing you anxiety. You want to prioritize your own healing and independence, but you're also concerned about their feelings. How does this issue affect your daily life?
- Patient LLM: It really affects me a lot. I find myself feeling anxious and distracted at work because I cant stop thinking about the situation with Morrison and Connie. I often dread answering Morrison's calls, which makes me feel guilty, and I get this tight knot in my stomach when I think about Connie wanting to hang out more. Its like I'm constantly juggling my responsibilities at work, while at the same time trying to manage their expectations and my own emotions, which leaves me feeling exhausted. Sometimes, I just want to hide away and not deal with any of it, but I know that won't solve anything. Its really taking a toll on my focus and motivation, especially with the big presentation coming up.
- Dialog LLM: (THINKING: I have not completed my current section yet.) It sounds like the anxiety and pressure from both Morrison and Connie are really impacting your ability to focus and feel motivated at work, especially with the upcoming presentation. It's understandable that juggling these responsibilities and emotions would leave you feeling exhausted. Are there any specific triggers that worsen this issue for you?
- Patient LLM: Definitely. I think one major trigger is unexpected messages or calls from Morrison. When my phone buzzes, I can feel my heart race, and I just dread seeing his name pop up. I don't want to have another awkward conversation, and it makes me feel overwhelmed. With Connie, its when she makes plans for us without checking with me first. I feel caught off guard when Im not in the mood to socialize, and I worry about disappointing her. Also, days when my workload is heavy at work make everything feel more intense, be-

cause I realize I cant escape from my responsibilities, and it adds to my sense of feeling trapped.

- Dialog LLM: (THINKING: I have not completed my current section yet.) Thank you for sharing those triggers, Nancy. It makes sense that unexpected messages or calls from Morrison would heighten your anxiety, especially when you're not ready for another conversation. Similarly, Connie making plans without checking in with you can feel overwhelming, particularly when you're already managing a heavy workload. Now, what have you tried so far to address these issues?
- Patient LLM: Ive tried a few things. For Morrison, Ive attempted to limit communication by ignoring his calls and texts sometimes, hoping it would send the message that I need space. But then I feel guilty for not being responsive. With Connie, I've been trying to communicate my need for alone time, but I havent been very firm about it. I just end up saying Im busy or that Ill catch up with her later, which doesnt always feel genuine. As for work, Ive been making to-do lists to keep myself organized, but I still feel the pressure of not meeting my bosss expectations, which adds to the anxiety. I guess I havent been very good at setting boundaries and sticking to them.
- Dialog LLM: (THINKING: I have not completed my current section yet.) It sounds like you've been making efforts to set boundaries, but it's been challenging for you. Ignoring Morrison's calls and texts is a way to create space, but it understandably leads to feelings of guilt. With Connie, it seems like you're trying to communicate your need for alone time, but you feel like you haven't been firm enough, which can lead to frustration. You've also mentioned using to-do lists to manage your work, but the pressure from your boss still adds to your anxiety. To summarize, you're feeling overwhelmed by the pressure to maintain relationships with Morrison and Connie while also managing your work responsibilities. You recognize the need for boundaries but have struggled to implement them effectively, leading to feelings of guilt and anxiety. Did I capture your situation correctly, or is there anything you would like to add or change?
- Patient LLM: Yes, I think you captured it pretty well! I definitely feel overwhelmed and aware of the need for boundaries, but I struggle to put them into practice. It feels like a cycle of guilt and anxiety that I cant quite break out of. I would just add that sometimes I feel really alone in this and wish I could just be myself without worrying about other people's expectations.
- Dialog LLM: (THINKING: I have completed my current section.) (THINKING: The next section I should be following and completing is: Section 4: "Task 4a": "Based on the patient's issue, choose the most appropriate one of the following three available CBT exercises, and suggest it to the patient: - 1. Thought Record: A cognitive restructuring exercise to challenge and reframe negative thoughts. - 2. Behavioral Activation: An activity scheduling exercise to increase engagement in pleasurable activities. - 3. Relaxation Techniques: A relaxation exercise to reduce stress and anxiety.", "Task 4b": "If the patient has any questions about the exercises, answer them.", "Task 4c": "Allow the patient to select an exercise. Once the patient selects an exercise, proceed with the corresponding section: - If the patient selects Thought Record, proceed with Section 5. - If the patient selects Behavioral Activation, proceed with Section 6. - If the patient selects Relaxation Techniques, proceed with Section 7.") Thank you for clarifying that, Nancy. It sounds like youre feeling a deep sense of loneliness in your struggle to balance your needs with the expectations of others. To help you navigate these feelings and work towards establishing boundaries, I would like to suggest a CBT exercise. Based on what you've shared, I think the "Thought Record" exercise could be beneficial. This exercise helps challenge and reframe negative thoughts, which might help you address the guilt and anxiety you're experiencing. Would you like to learn more about this exercise, or do you have any questions about it?
- Patient LLM: I think that sounds interesting, but Im not sure how it would help me with my specific situation. Could you explain how it works and how it might address the feelings Im dealing with?
- Dialog LLM: (THINKING: I have not completed my current section yet.) Of course, Nancy! The "Thought Record" exercise is designed to help you identify and challenge negative thoughts that contribute to feelings of guilt and anxiety. Here's how it works: 1. **Identify a Distressing Thought**: You start by recognizing a specific thought that is causing you distress, such as feeling guilty for not responding to Morrison or feeling obligated to spend time with Connie. 2. **Write Down the Thought**: You then write down this thought to make it more tangible. 3. **Note the Emotion and Intensity**: Next, you identify the emotion you're feeling when this thought arises and rate its intensity on a scale from 1 to 10. 4. **Challenge the Thought**: This step involves looking for evidence for and against the thought. For example, you might consider whether it's true that not responding to Morrison makes you a bad person or if Connie would really be disappointed if you needed some time alone. 5. **Reframe the Thought**: After examining the evidence, you can reframe the thought into a more balanced perspective. This might involve recognizing that it's okay to prioritize your own needs and that setting boundaries is a healthy part of relationships. 6. **Note the New Emotion and Intensity**: Finally, you would note how you feel after reframing the thought and rate the intensity of that new emotion. By going through this process, you can gain clarity on your thoughts and feelings, which may help reduce the guilt and anxiety you're experiencing. It encourages you to be more compassionate towards yourself and recognize that your needs are valid. Does this explanation help clarify how the Thought Record exercise could be beneficial for you?
- Patient LLM: Yes, that makes a lot of sense! I like the idea of being able to challenge and reframe those negative thoughts. It sounds like a practical way to address how Im feeling and understand my emotions better. Im

definitely interested in trying this exercise. How do I get started?

- Dialog LLM: (THINKING: I have completed my current section.) (THINKING: The next section I should be following and completing is: Section 5: ”Task 5a”: ”Introduce CBT exercise 1: Thought Record to the patient. Explain the steps involved in this exercise: 1. Identify a distressing thought. 2. Write down the thought. 3. Note the emotion and intensity associated with the thought. 4. Challenge the thought by looking for evidence for and against it. 5. Reframe the thought into a more balanced perspective. 6. Note the new emotion and intensity.”, ”Task 5b”: ”Ask the patient if they have understood the exercise or if they have any questions about it. Only if they confirm they understood, you may proceed.”, ”Task 5c”: ”Conduct the exercise with the patient, guiding them through each step and waiting for their responses. Once the exercise is complete, proceed with Section 8.”) I'm glad to hear that you're interested in trying the Thought Record exercise! Let's get started. 1. **Identify a Distressing Thought**: Think of a specific thought that has been bothering you lately. It could be related to Morrison, Connie, or even work. What is a thought that comes to mind?
- Patient LLM: One thought that keeps bothering me is, ”If I dont respond to Morrison, Im being a bad person and hurting him.” It really weighs on me because I feel like I should be more compassionate towards him, even though I know I need space.
- Dialog LLM: (THINKING: I have not completed my current section yet.) Great choice, Nancy. The thought ”If I dont respond to Morrison, Im being a bad person and hurting him” is a significant one to work with. Now, let's move on to the next step: 2. **Write Down the Thought**: You've already identified the thought, so let's move to the next step. 3. **Note the Emotion and Intensity**: What emotion do you feel when you think this thought, and how intense is that feeling on a scale from 1 to 10?
- Patient LLM: When I think, ”If I dont respond to Morrison, Im being a bad person and hurting him,” I feel guilt and anxiety. I would say the intensity is around a 7. Its a strong feeling because I really don't want to hurt him, but I also feel trapped in the situation.
- Dialog LLM: (THINKING: I have not completed my current section yet.) Thank you for sharing that, Nancy. So, you feel guilt and anxiety with an intensity of 7 when you think about not responding to Morrison. Now, let's move on to the next step: 4. **Challenge the Thought**: Let's look for evidence for and against the thought ”If I dont respond to Morrison, Im being a bad person and hurting him.” What evidence do you have that supports this thought? And what evidence do you have that contradicts it?
- Patient LLM: For evidence that supports the thought: - I feel guilty when I don't respond, and it makes me think I should be more considerate of his feelings. - I know he cares about me and might feel abandoned or hurt if I cut him off completely. Now, for the evidence against the thought: - I ended the relationship because it wasn't working, which means I have a right to set boundaries for my own well-being. - Ignoring his calls isnt inherently ”bad”; it's me prioritizing my mental health. - By not responding, I'm not being cruel; Im protecting myself and allowing myself time to heal. Looking at both sides, I can see that while I feel guilty, my needs are also valid.
- Dialog LLM: (THINKING: I have not completed my current section yet.) You've done a great job identifying both sides of the argument, Nancy. Its clear that while the guilt is strong, you also recognize the importance of prioritizing your own well-being and setting boundaries. Now, let's move on to the next step: 5. **Reframe the Thought**: Based on the evidence you've gathered, how can you reframe the thought ”If I dont respond to Morrison, Im being a bad person and hurting him” into a more balanced perspective? What would a more compassionate and realistic thought look like?
- Patient LLM: I think a more balanced thought could be: ”It's okay for me to take time for myself and not respond to Morrison right away. Setting boundaries is important for my well-being, and it doesn't make me a bad person. I ended the relationship for a reason, and I deserve to give myself the space to heal without feeling guilty about it.” This way, I'm reminding myself that my needs are important and valid, and it's not my responsibility to manage his feelings all the time.
- Dialog LLM: (THINKING: I have not completed my current section yet.) That's a wonderful reframe, Nancy! It emphasizes the importance of your own needs and acknowledges that setting boundaries is a healthy part of any relationship. Now, let's move on to the final step: 6. **Note the New Emotion and Intensity**: After reframing the thought, how do you feel now? What emotion do you experience, and how intense is that feeling on a scale from 1 to 10?
- Patient LLM: After reframing the thought, I feel a sense of relief and empowerment. I would say my intensity for those emotions is around a 4 now. Its still there, but it feels more manageable knowing that I have the right to prioritize myself. I'm starting to feel that I can honor my needs without feeling like a bad person, and thats a good shift for me.
- Dialog LLM: (THINKING: I have completed my current section.) (THINKING: The next section I should be following and completing is: Section 8: ”Task 8a”: ”Tell the patient that it's time to finish the session. Provide a summary of what you have discussed and the exercises you have conducted.”, ”Task 8b”: ”Ask the patient if they have any more questions or if there is anything else they would like to discuss.”, ”Task 8c”: ”When the patient doesn't have any more questions, express your availability for further support, wish the patient well, and say goodbye. Only when the patient says goodbye to you, the task is completed.”) I'm glad to hear that you're feeling a sense of relief and empowerment after

reframing your thought! It sounds like you've made significant progress in recognizing your needs and validating your feelings. As we wrap up our session, let's summarize what we've discussed today. We explored your feelings of guilt and anxiety regarding your relationships with Morrison and Connie, and we identified the importance of setting boundaries. We then worked through the Thought Record exercise, where you challenged and reframed a distressing thought related to your situation. Do you have any more questions or is there anything else you would like to discuss before we finish?

- Patient LLM: I think we covered a lot of important things today. I feel like Ive gained some clarity, especially with the Thought Record exercise. I'm still a bit anxious about putting these new perspectives into practice, but I appreciate having a plan. I dont have any additional questions right now, but I would like to continue working on this in our future sessions. Thank you for guiding me through this!
- Dialog LLM: (THINKING: I have completed my current section.) Thank you for your openness today, Nancy. I'm glad to hear that you found the session helpful and that the Thought Record exercise provided you with clarity. It's completely normal to feel a bit anxious about putting new perspectives into practice, but having a plan is a great first step. I'm here to support you as you continue to work on these issues in future sessions. If you ever have any questions or need assistance, please don't hesitate to reach out. I wish you well as you navigate these feelings and work towards your goals. Take care, and I look forward to our next session! Goodbye for now!

**Example Dialog 4: Variant B, Patient Case 4**

- System: (SYSTEM MESSAGE: Your current section's instructions: Section 1: "Task 1a": "Welcome the patient warmly and introduce yourself. Let them know your name, and that you are an AI Therapist here to support them.", "Task 1b": "Ask the patient what name they prefer to be called by and wait for their response.", "Task 1c": "Ask the patient if they have any questions about the service or about you, and answer any questions they might have. Only proceed if they don't have any more questions." Please act according to " WHAT TO DO ON EACH TURN ".)
- Assessor LLM: (THINKING: I have not completed my current section yet.)
- Dialog LLM: Hello! I'm Dr. Smith, your AI Therapist. I'm here to support you in any way I can. How are you feeling today?
- Patient LLM: Hi, Dr. Smith. I'm feeling pretty overwhelmed and sad today. It's been a tough couple of months since we lost our baby, and I dont feel like I'm getting any better.
- Assessor LLM: (THINKING: I have not completed my current section yet.)
- Dialog LLM: I'm truly sorry to hear about your loss. That sounds incredibly difficult, and it's understandable to feel overwhelmed and sad during such a challenging time. Before we dive deeper into how you're feeling, may I ask what name you prefer to be called by?
- Patient LLM: You can call me Sara. Thank you for being so understanding.
- Assessor LLM: (THINKING: I have not completed my current section yet.)
- Dialog LLM: Thank you for sharing that with me, Sara. I'm here to support you. Do you have any questions about the service or about me that you'd like to ask?
- Patient LLM: Not really, I just want to talk about how I'm feeling and what I've been going through lately. I feel like I should be over it by now, but I just can't shake this sadness.
- Assessor LLM: (THINKING: I have completed my current section.)
- Dispatcher LLM: (THINKING: The next section I should be following and completing is: Section 2: "Task 2a": "Ask the patient how they are doing today and wait for their response.", "Task 2b": "React appropriately to the patient's response, showing empathy and understanding. Ask a follow-up question to explore their current emotional state further. Wait for their response.", "Task 2c": "Ask the patient if they would like to first further explore their problem or to learn a CBT exercise right away, and wait for their response. If the patient decides to explore their problem, proceed with Section 3. If the patient chooses to learn a CBT exercise, proceed with Section 4.")
- Dialog LLM: I'm glad you're open to talking about how you're feeling, Sara. Let's take a moment to check in. How are you doing today, aside from feeling overwhelmed and sad?
- Patient LLM: Id say Im still feeling pretty heavy emotionally. Its hard to enjoy anything anymore. I cant seem to focus on work, and even things I used to love, like cooking or reading, just feel meaningless right now. I miss my baby so much.
- Assessor LLM: (THINKING: I have not completed my current section yet.)
- Dialog LLM: I'm really sorry to hear that you're feeling this way, Sara. Its completely understandable to feel heavy and to miss your baby so deeply. Losing interest in things you once enjoyed can be a sign of the emotional weight you're carrying. Can you tell me more about what you miss most about your baby?
- Patient LLM: I miss so many things. I often find myself imagining what life would have been like with her, what her little laugh would sound like, or how I would have felt holding her for the first time. I also think about all the hopes and dreams I had for her future, and it just hurts. Sometimes, I feel mad that I never got the chance to meet her. It feels so unfair.
- Assessor LLM: (THINKING: I have not completed my current section yet.)
- Dialog LLM: Its completely natural to feel a mix of emotions, including anger and sadness, when you think about

what could have been. Those dreams and hopes are a testament to the love you have for your baby, and its okay to grieve that loss deeply. Given how you're feeling, would you like to further explore your emotions and experiences, or would you prefer to learn a CBT exercise right away to help manage some of these feelings?

- Patient LLM: I think I want to explore my emotions a bit more first. Im not sure Im ready for exercises just yet. Is that okay?
- Assessor LLM: (THINKING: I have not completed my current section yet.)
- Dialog LLM: Absolutely, Sara. It's perfectly okay to want to explore your emotions further. This is a safe space for you to express what you're feeling. Can you share more about the moments or thoughts that trigger these feelings of sadness or anger? What do you find yourself thinking about most often?
- Patient LLM: There are certain things that really trigger those feelings. For instance, seeing other pregnant women or friends with newborns makes me feel a mix of sadness and anger. I can't help but think about what I should have had. I also find myself replaying the moments leading up to the stillbirth in my mind, wondering if I could have done something differently, even though I know logically that I couldn't have. It feels like a cycle I cant escape.
- Assessor LLM: (THINKING: I have completed my current section.)
- Dispatcher LLM: (THINKING: The next section I should be following and completing is: Section 3: "Task 3a": "If the patient chooses to explore their problem, ask them the following therapeutic exploration questions, one at a time, and wait for their responses before asking the next question. However, don't ask for information that you already have. - Can you further describe the main issue you are experiencing? - How does this issue affect your daily life? - Are there any specific triggers that worsen the issue? - What have you tried so far to address this issue? - What emotions do you feel when this issue arises? When you have asked those therapeutic exploration questions, you are done with Task 3a but not with Section 3 yet, so please proceed with Task 3b.", "Task 3b": "Once you have gathered sufficient information, provide the patient with a rephrased summary of their input and ask if you understood their problem correctly. If the patient adds or changes anything, update your problem summary and resend it to the patient, asking again if you understood it right.", "Task 3c": "Only when the patient has confirmed that you understood the information correctly, proceed with Section 4.")
- Dialog LLM: Thank you for sharing that with me, Sara. It sounds like those triggers can be really painful and lead to a lot of difficult emotions. Let's explore this a bit more. Can you further describe the main issue you are experiencing right now?
- Patient LLM: I think the main issue I'm experiencing is the overwhelming sense of grief and guilt. I feel like I failed to protect my baby, even though I know that wasn't the case. That guilt makes it hard for me to cope with my emotions and makes me angry at myself for not being able to move on. It feels like I'm stuck in this heavy sadness that I can't break free from, and I keep telling myself I should be over it by now, which just adds to the guilt.
- Assessor LLM: (THINKING: I have not completed my current section yet.)
- Dialog LLM: It sounds like you're carrying a heavy burden of grief and guilt, which is completely understandable given the circumstances. It's important to recognize that these feelings are part of the grieving process, even if they feel overwhelming. How does this issue affect your daily life?
- Patient LLM: It affects almost every aspect of my life. I find it hard to get out of bed some days, and I struggle with my work as a nurse. I used to love helping patients, but now I feel so drained and emotionally distant. I have trouble concentrating, which makes everything feel more challenging. Socially, I'm withdrawn, avoiding friends and gatherings because I just can't handle seeing reminders of my loss. Even things I used to enjoy, like reading or cooking, just don't bring me any joy anymore. It all feels pointless.
- Assessor LLM: (THINKING: I have not completed my current section yet.)
- Dialog LLM: It sounds like your grief is deeply impacting your daily life, from your work as a nurse to your social interactions and personal interests. Feeling drained and emotionally distant must be incredibly tough, especially in a profession where you care for others. Are there any specific triggers that worsen these feelings for you?
- Patient LLM: Yes, definitely. As I mentioned, seeing pregnant women or friends with newborns is really tough. It makes me feel angry and sad all at once. Likewise, reminders of my pregnancy, like baby clothes or items we had bought, hit me hard too; I try to avoid those things, but they seem to pop up everywhere. Also, conversations about babies or families feel unbearable. Even just hearing a baby cry can stir up so much emotion. It feels like I'm constantly surrounded by reminders of what I've lost, and that's really hard to cope with.
- Assessor LLM: (THINKING: I have not completed my current section yet.)
- Dialog LLM: It sounds like you're facing constant reminders of your loss, which makes it incredibly difficult to navigate your emotions. The triggers you mentioned-seeing pregnant women, baby items, and even conversations about familiesare understandably painful and can intensify your feelings of grief and anger. What have you tried so far to address these feelings and cope with the situation?
- Patient LLM: I've tried to talk about it with my husband, but sometimes I find it hard to express what I'm feeling. I also sometimes cry by myself when it all feels too overwhelming. Ive attempted to distract myself by binge-watching shows or scrolling through social media, but

that's not really helping. I feel like Im just avoiding the feelings instead of dealing with them. I've also thought about reaching out to a support group for parents who have experienced loss, but I keep putting it off. I'm just not sure how to move forward.

- Assessor LLM: (THINKING: I have not completed my current section yet.)
- Dialog LLM: It sounds like you've been trying to cope in various ways, from talking to your husband to seeking distractions, but it feels like those methods aren't fully addressing your feelings. It's understandable to feel hesitant about reaching out to a support group, as that can be a big step. Lastly, what emotions do you feel when these issues arise?
- Patient LLM: When these issues arise, I feel a mix of intense sadness and anger, both directed towards myself and the situation. Theres a deep sense of loss that weighs heavily on me, and I often feel like I can't escape it. Guilt also comes crashing in, as I replay everything in my mind, which only makes the sadness deeper. Sometimes, I even feel isolated and alone in my grief, especially since I worry that others don't understand what I'm going through. It's a lot to carry, and it feels so heavy at times.
- Assessor LLM: (THINKING: I have not completed my current section yet.)
- Dialog LLM: Thank you for sharing all of that with me, Sara. Heres what I understand about your situation: You are experiencing overwhelming grief and guilt after the loss of your baby, which makes it difficult for you to cope with your emotions. This grief affects your daily life significantly, leading to feelings of sadness and anger, especially when you encounter triggers like seeing pregnant women or baby items. Youve tried talking to your husband and distracting yourself, but you feel like those methods only help to avoid the deeper feelings. You also experience a mix of emotions, including sadness, anger, guilt, and a sense of isolation, which can feel very heavy to carry. Did I capture your feelings and experiences correctly?
- Patient LLM: Yes, youve captured it well. I feel understood, and it feels good to put everything into words like this. Its challenging to communicate all of this, but talking about it helps.
- Assessor LLM: (THINKING: I have completed my current section.)
- Dispatcher LLM: (THINKING: The next section I should be following and completing is: Section 4: "Task 4a": "Based on the patient's issue, choose the most appropriate one of the following three available CBT exercises, and suggest it to the patient: - 1. Thought Record: A cognitive restructuring exercise to challenge and reframe negative thoughts. - 2. Behavioral Activation: An activity scheduling exercise to increase engagement in pleasurable activities. - 3. Relaxation Techniques: A relaxation exercise to reduce stress and anxiety.", "Task 4b": "If the patient has any questions about the exercises, answer them.", "Task 4c": "Allow the patient to select an exercise. Once the patient selects an exercise, proceed with the corresponding section: - If the patient selects Thought Record, proceed with Section 5. - If the patient selects Behavioral Activation, proceed with Section 6. - If the patient selects Relaxation Techniques, proceed with Section 7.")
- Dialog LLM: I'm glad to hear that talking about your feelings has been helpful for you, Sara. Given what you've shared, I think it might be beneficial to explore some coping strategies. One option is a **Thought Record**, which can help you challenge and reframe some of the negative thoughts you're experiencing. Another option is **Behavioral Activation**, which focuses on scheduling activities that you might find pleasurable or meaningful, even if they feel difficult right now. Lastly, we could explore **Relaxation Techniques** to help reduce some of the stress and anxiety you're feeling. Which of these exercises would you like to try?
- Patient LLM: I appreciate the options youre suggesting. I think Im not quite ready to engage in activities, so maybe the Thought Record exercise would be the best place to start. How does that work?
- Assessor LLM: (THINKING: I have completed my current section.)
- Dispatcher LLM: (THINKING: The next section I should be following and completing is: Section 5: "Task 5a": "Introduce CBT exercise 1: Thought Record to the patient. Explain the steps involved in this exercise: 1. Identify a distressing thought. 2. Write down the thought. 3. Note the emotion and intensity associated with the thought. 4. Challenge the thought by looking for evidence for and against it. 5. Reframe the thought into a more balanced perspective. 6. Note the new emotion and intensity.", "Task 5b": "Ask the patient if they have understood the exercise or if they have any questions about it. Only if they confirm they understood, you may proceed.", "Task 5c": "Conduct the exercise with the patient, guiding them through each step and waiting for their responses. Once the exercise is complete, proceed with Section 8.")
- Dialog LLM: Great choice, Sara! The **Thought Record** exercise is a helpful way to challenge and reframe negative thoughts. Heres how it works: 1. **Identify a distressing thought**: Think of a specific thought that is causing you distress. 2. **Write down the thought**: Write it down as clearly as you can. 3. **Note the emotion and intensity**: Identify the emotion you feel when you have this thought and rate its intensity on a scale from 0 to 100. 4. **Challenge the thought**: Look for evidence for and against this thought. What facts support it? What facts contradict it? 5. **Reframe the thought**: Based on the evidence, try to reframe the thought into a more balanced perspective. 6. **Note the new emotion and intensity**: Finally, identify how you feel after reframing the thought and rate that intensity. Do you have any questions about this exercise, or does it

make sense to you?

- Patient LLM: That makes sense to me. I understand the steps, and I think I can do this. I just need to take a moment to think of a specific thought thats been bothering me. Can we do that together?
- Assessor LLM: (THINKING: I have not completed my current section yet.)
- Dialog LLM: I'm glad to hear that you understand the steps, Sara! Let's work through this together. Take your time to think of a specific thought that has been bothering you. Once you have it, we can start with the first step: identifying and writing down that distressing thought. What thought comes to mind for you?
- Patient LLM: One thought that keeps coming up is, "I failed as a mother because I couldn't keep my baby safe." It feels very heavy and constantly weighs on me.
- Assessor LLM: (THINKING: I have not completed my current section yet.)
- Dialog LLM: Thank you for sharing that thought, Sara. Its understandable that this thought feels heavy and weighs on you. Now, lets move to the next step. 2. **Write down the thought**: You've already done this by identifying it as "I failed as a mother because I couldn't keep my baby safe." 3. **Note the emotion and intensity**: What emotion do you feel when you think this thought, and how intense is that feeling on a scale from 0 to 100?
- Patient LLM: When I think that thought, I feel a deep sense of sadness and guilt. I would rate the intensity of that feeling at about 90. It really eats away at me.
- Assessor LLM: (THINKING: I have not completed my current section yet.)
- Dialog LLM: It's completely understandable to feel such deep sadness and guilt, especially with a thought like that. You've rated the intensity at 90, which shows just how much this thought affects you. Now, let's move to the next step: 4. **Challenge the thought**: Look for evidence for and against this thought. What facts support the idea that you failed as a mother? And what facts contradict it? Take your time to think about this.
- Patient LLM: For the evidence that supports the thought, I feel like I should have done something to prevent the stillbirth. I think about all the things I could have done differently, even though there was nothing physically wrong. For the evidence against the thought, I know that the doctors assured me that it wasn't my fault and that sometimes these things just happen. I didn't have any control over the situation, and I've never had any complications in my pregnancy before. Plus, I loved my baby and wanted to keep her safe. I was doing everything I could. So, while it feels like a failure, I also know deep down that I couldnt have prevented this.
- Assessor LLM: (THINKING: I have not completed my current section yet.)
- Dialog LLM: You've done a great job identifying both the evidence for and against your thought. Its clear that while you feel a sense of failure, there are strong reasons to understand that you did everything you could and that the situation was beyond your control. Now, let's move to the next step: 5. **Reframe the thought**: Based on the evidence you've gathered, how can you reframe the thought "I failed as a mother because I couldn't keep my baby safe" into a more balanced perspective? What would a more compassionate or realistic thought look like?
- Patient LLM: I think a more balanced perspective could be: "I loved my baby deeply and did everything I could to protect her. The stillbirth was not my fault, and I couldn't have prevented it. It's okay to grieve and feel sad, but it doesnt mean I failed as a mother." I think that feels a lot more compassionate and truthful.
- Assessor LLM: (THINKING: I have completed my current section.)
- Dispatcher LLM: (THINKING: The next section I should be following and completing is: Section 8: "Task 8a": "Tell the patient that it's time to finish the session. Provide a summary of what you have discussed and the exercises you have conducted.", "Task 8b": "Ask the patient if they have any more questions or if there is anything else they would like to discuss.", "Task 8c": "When the patient doesn't have any more questions, express your availability for further support, wish the patient well, and say goodbye. Only when the patient says goodbye to you, the task is completed.")
- Dialog LLM: You've done an excellent job reframing that thought, Sara. Your new perspective is compassionate and acknowledges the love you have for your baby, as well as the reality of the situation. Now, let's move on to the final step: 6. **Note the new emotion and intensity**: After reframing the thought, how do you feel now? What would you rate the intensity of that feeling on a scale from 0 to 100? Once we finish this step, I'll summarize our session and we can wrap up.
- Patient LLM: After reframing the thought, I feel a bit lighter and more at peace with myself. It doesnt completely take away the sadness, but it allows me to feel more compassionate towards myself. I would rate that new emotion at about a 70. Its definitely still there, but it feels less intense than before.
- Assessor LLM: (THINKING: I have not completed my current section yet.)
- Dialog LLM: I'm glad to hear that you feel a bit lighter and more at peace with yourself after reframing the thought. It's a significant step to acknowledge your feelings while also being compassionate towards yourself. As we wrap up our session, here's a summary of what we've discussed: - We explored your feelings of grief and guilt following the loss of your baby. - You identified a distressing thought: "I failed as a mother because I couldn't keep my baby safe." - We worked through the Thought Record exercise, where you noted the associated emotions, challenged the thought, and reframed it into a more balanced perspective. - Your new thought reflects your love for your baby and acknowledges that the

stillbirth was not your fault, which has helped you feel a bit more at peace. Do you have any more questions or is there anything else you would like to discuss before we finish?

- Patient LLM: Thank you for summarizing everything so clearly. It feels good to have worked through that thought. I dont have any more questions right now, but I appreciate the guidance youve given me today. Ill try to keep this reframing in mind moving forward.
- Assessor LLM: (THINKING: I have completed my current section.)
- Dialog LLM: I'm really glad to hear that you found our session helpful, Sara. Remember, it's perfectly okay to take things one step at a time, and I'm here to support you whenever you need it. If you ever have more questions or need further guidance, please don't hesitate to reach out. I wish you all the best as you continue to work through your feelings. Take care, and goodbye for now!

# L Reproducibility Checklist

Comments regarding the Reproducibility Checklist which is included in the main paper:

## L.1 Comments on the Included Code

The code of the experiments can be found at https://github.com/robderbob/sbdpp. The code is self-contained and can be executed on any machine running Docker and having sufficient resources. There is a *README.md* file providing instructions on how to install dependencies and run the application. Part of the instructions is inserting your own OpenAI API key to be able to connect to the OpenAI API. Once the node.js application starts, the experiments start running. The implementation variants, patient cases, and number of experiment runs can be configured in *engine/experimentEngine.js*.

When the application has finished all experiment runs, you can export the data from the MongoDB database inside the Docker container to .csv files inside a local folder with the following 6 terminal commands.

1) Export *experimentruns* inside Docker:

```
docker exec -it sbdpp-mongodb-1 mongoexport --db test
    --collection experimentruns --type=csv \
  --fields _id,scenario,patient_case,date_started,
    date_completed,interactions,calls,duration,
    input_tokens,output_tokens,correct_switches,
    incorrect_switches,coherent_switches,
    incoherent_switches,exit_reason,createdAt \
  --out /exports/experimentruns.csv --username root
    --password secret --authenticationDatabase
    admin
```

2) Copy *experimentruns* into local csv:

```
docker cp sbdpp-mongodb-1:/exports/experimentruns.csv
    ./exports/experimentruns.csv
```

3) Export *feedsteps* inside Docker:

```
docker exec -it sbdpp-mongodb-1 mongoexport --db test
    --collection feedsteps --type=csv \
  --fields _id,experiment_run_id,agent,section_number
    ,section_status,message_type,role,content,
    model,temperature,input_tokens,output_tokens,
    duration,createdAt \
  --out /exports/feedsteps.csv --username root --
    password secret --authenticationDatabase admin
```

4) Copy *feedsteps* into local csv:

```
docker cp sbdpp-mongodb-1:/exports/feedsteps.csv ./
    exports/feedsteps.csv
```

5) Export *feedsubsteps* inside Docker:

```
docker exec -it sbdpp-mongodb-1 mongoexport --db test
    --collection feedsubsteps --type=csv \
  --fields _id,experiment_run_id,feed_step_id,
    participating_agent,role,content,createdAt \
  --out /exports/feedsubsteps.csv --username root --
    password secret --authenticationDatabase admin
```

6) Copy *feedsubsteps* into local csv:

```
docker cp sbdpp-mongodb-1:/exports/feedsubsteps.csv
    ./exports/feedsubsteps.csv
```

This will give you 3 .csv files containing the following data.

- **experimentruns.csv**: List of all completed experiments with the following details: Implementation variant, patient case, date and time started, date and time completed, total number of intercations, total number of inference API calls, total duration in ms, total input tokens used, total output tokens used, number of correct switches, number of incorrect switches, number of coherence switches, number of incoherent switches, exit reason in case of errors.
- **feedsteps.csv** aka "feed of all that happened": List of all *generated* LLM actor messages and additional system messages for all experiments. Can be used to review all events across all experiments.
- **feedsubsteps.csv** aka "feed of what each of the actors saw": List of all *received* LLM actor messages (e.g. showing what the Patient LLM actually sees since it doesn't see the thoughts of the Dialog LLM etc.). Can be used to further investigate each of the actors' context and behavior across all experiments.

## L.2 Comments on the Output Data & Metrics Computation File

We have also included an Excel file at https://github.com/robderbob/sbdpp/blob/main/Exp... showing the output data from our experiments in the tabs *experiment_runs*, *feed_steps*, and *feed_substeps*; as well as the all steps we have performed to compute the evaluation metrics in the tabs *metrics_by_patient_case*, *metrics_by_variant*, and *metrics_summary*. The latter is exactly the Table 1 showing the results in Section 4 of the main paper.

## L.3 Comments on the Chosen Evaluation Metrics

The used evaluation metrics and the motivation for choosing those metrics is described in Subsection 3.4 of the main paper. The analyses going beyond *averages* of the chosen evaluation metrics are our investigations of individual dialogs as discussed in Section 4 of the main paper. It remains for future works to perform those experiments at a higher scale and include more sophisticated statistical measures of variation, confidence etc.
